# Supplementary material for: Hide in Thicket: Generating Imperceptible and Rational Adversarial Perturbations on 3D Point Clouds
Source: arXiv:2403.05247 source file (2024-03-08)
Supplement: Supplementary file 1 [file X_suppl.tex]

\clearpage
\setcounter{page}{1}
\maketitlesupplementary

% \section{Rationale}
% \label{sec:rationale}
% % 
% Having the supplementary compiled together with the main paper means that:
% % 
% \begin{itemize}
% \item The supplementary can back-reference sections of the main paper, for example, we can refer to \cref{sec:intro};
% \item The main paper can forward reference sub-sections within the supplementary explicitly (e.g. referring to a particular experiment); 
% \item When submitted to arXiv, the supplementary will already included at the end of the paper.
% \end{itemize}
% % 
% To split the supplementary pages from the main paper, you can use \href{https://support.apple.com/en-ca/guide/preview/prvw11793/mac#:~:text=Delete%20a%20page%20from%20a,or%20choose%20Edit%20%3E%20Delete).}{Preview (on macOS)}, \href{https://www.adobe.com/acrobat/how-to/delete-pages-from-pdf.html#:~:text=Choose%20%E2%80%9CTools%E2%80%9D%20%3E%20%E2%80%9COrganize,or%20pages%20from%20the%20file.}{Adobe Acrobat} (on all OSs), as well as \href{https://superuser.com/questions/517986/is-it-possible-to-delete-some-pages-of-a-pdf-document}{command line tools}.

In the manuscript, we detail the proposed HiT-ADV deformation attack framework and provide a wealth of experimental results. 
In the supplementary materials, we add more details and results, specifically including:

\begin{itemize}
\item We introduce the detailed hyper-parameter settings for HiT-ADV.

\item We present more ablation study results for comprehensive understanding.

\item We present the comparison of visualization results under the setting of targeted attacks.

\item We supplement the comparison of visualized results of various attack methods on other datasets and models.
\end{itemize}

\section{Detailed Settings for HiT-ADV}
The proposed HiT-ADV is implemented based on the C\&W attack framework~\cite{carlini2017cw}, which uses a hyper-parameter $\lambda$ to balance the trade-off relationship between adversarial strength and imperceptibility. 
Following the C\&W framework, we also conduct a binary search for $\lambda$, setting its initial value at $10$, with a maximum of $80$ and a minimum of $0$. 
If the search for $\lambda$ reaches $0$ and the prediction is still $y$, we consider it a failed attack.
Furthermore, we use a margin threshold $\kappa$ in the classification loss function to measure the required level of adversarial strength, which is set as $30$ by default.

In the two-stage attack region search module of the specific HiT-ADV framework, we use three adjustable hyper-parameters, namely, the number of candidate center points $n$ sampled through farthest points sampling, the number of local points $k$ gathered around the center point, and finally, the number of ultimate center points $\tilde{n}$ selected based on the SI score $\mathcal{S}$.
For the hyper-parameters $n$ and $k$, the principle of their setting is that the product of $n$ and $k$ should be close to the number of points in the input point cloud. 
For instance, for the ModelNet40 dataset, in the quantitative experiments of this paper, we use point clouds of $1024$ points as input, hence $n$ and $k$ are set to $100$ and $10$, respectively; in the qualitative experiments, we use all $10000$ points of each point cloud as input, therefore $n$ and $k$ are set to $100$ and $100$, respectively.
As for $\tilde{n}$, it reflects the global extent of the deformation perturbations. 
Specifically, the larger $\tilde{n}$ is, the more evenly the deformation perturbations will occur in each part; the smaller $\tilde{n}$ is, the more the deformation perturbations will concentrate in areas less sensitive to the human eye. 
In this paper, $\tilde{n}$ is set to $50$ by default.

During the process of iterative attacks, our framework also involves some hyper-parameters, including $a$, $\lambda_1$, $\lambda_2$, and $\lambda_3$.
$a$ limits the maximum value of $\sigma$ in all Gaussian kernel functions, it is a part of $\mathcal{L}_{ker}$, and describes the constraint on the shape of the Gaussian kernel functions.
In this paper, $a$ is set to $1.5$ by default.
As for $\lambda_1$, $\lambda_2$, and $\lambda_3$, they measure the emphasis of the attack on each regularization term. In this paper, we set them by default to $1$, $1$, $0.1$.

Although it seems that there are quite a few hyperparameters to set in our method, many of them can actually be automatically optimized through binary search, just like $\lambda$, but this process introduces greater time costs. 
Therefore, we simply set them manually in experiments. 
In fact, in most tasks, using the default parameters we provide can already achieve very superior performance.
\section{Supplement to Ablation Study}

\begin{figure}[t]
  \centering
  % \fbox{\rule{0pt}{2in} \rule{0.9\linewidth}{0pt}}
   \includegraphics[width=1\linewidth]{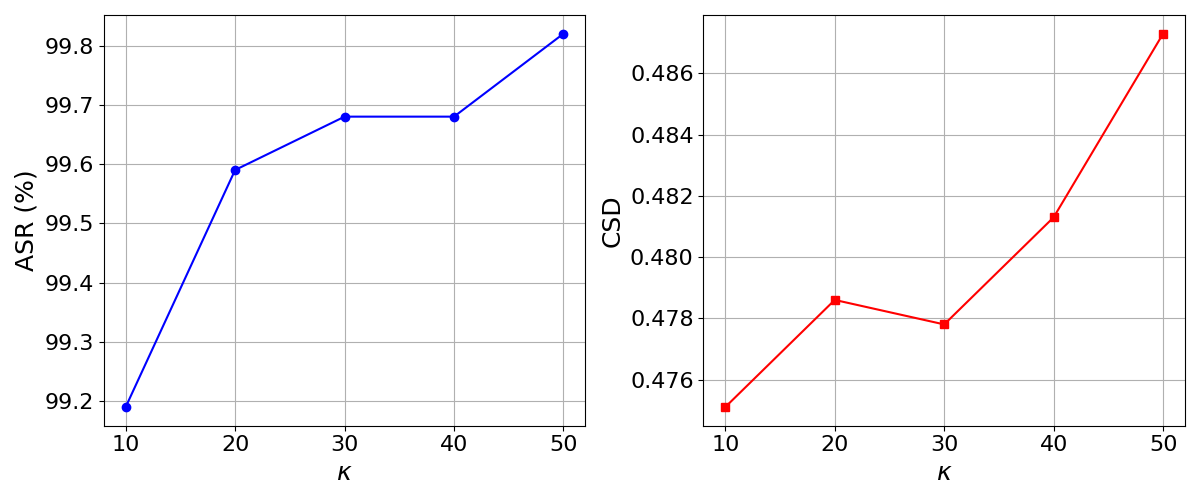}
   \caption{The influence of the hyper-parameter $\kappa$ in $\mathcal{L}_{cls}$. We compare the different ASR and CSD distances of HiT-ADV under different $\kappa$ settings.}
   \label{fig:ablationkappa}
   \vspace{-1mm}
\end{figure}

\begin{figure}[t]
  \centering
  % \fbox{\rule{0pt}{2in} \rule{0.9\linewidth}{0pt}}
   \includegraphics[width=1\linewidth]{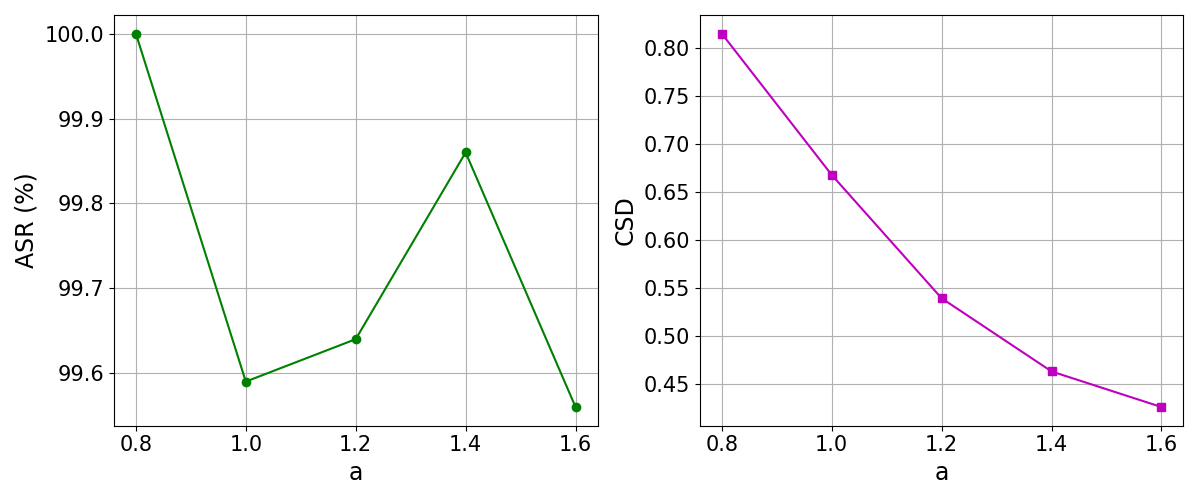}
   \caption{The influence of the hyper-parameter $a$ in $\mathcal{L}_{ker}$. We compare the different ASR and CSD distances of HiT-ADV under different $a$ settings.}
   \label{fig:ablationa}
   \vspace{-1mm}
\end{figure}

In this section, we conduct ablation experiments on two critical hyper-parameters, $\kappa$ and $a$, in HiT-ADV, and the results can be seen in Fig.~\ref{fig:ablationkappa} and Fig.~\ref{fig:ablationa} respectively.
In these two figures, we plot the trends of changes in ASR(\%) and CSD, two indicators representing adversarial strength and imperceptibility, respectively, as $\kappa$ and $a$ increase from small to large values.
It can be seen that as $\kappa$ increases, the optimization objective requires stronger adversarial strength, but at the cost of reduced imperceptibility.
When $a$ increases, HiT-ADV allows each Gaussian kernel function to be flatter, reducing the severe deformation perturbations, and therefore significantly lowering the CSD metric. 
However, this inevitably leads to a slight decrease in adversarial strength.
Thus, we empirically choose $1.5$ as the default value for $a$, to balance between adversarial strength and imperceptibility.

\section{Performance of Targeted Attacks}
Targeted attack is a more meaningful setup in physical scenarios. Since HiT-ADV itself is similar to the C\&W attack framework, it can be easily extended from an untargeted to a targeted setting following the C\&W approach. The visualization and comparison results are shown in Fig.~\ref{fig:target}.
Targeted attacks are more challenging as they require greater adversarial strength in the adversarial examples to achieve successful attacks.
It is easy to find that all three comparison methods are more perceptible compared to untargeted attacks: the point-based attacks 3D-ADV and GeoA$^3$ generate more outliers; HiT-ADV, on the other hand, requires larger deformation perturbations.
However, even though the degree of deformation in the targeted HiT-ADV has increased, its adversarial samples still maintain a reasonable shape, which validates the superior imperceptibility of HiT-ADV.

\begin{figure*}[t]
  \centering
  % \fbox{\rule{0pt}{2in} \rule{0.9\linewidth}{0pt}}
   \includegraphics[width=1\linewidth]{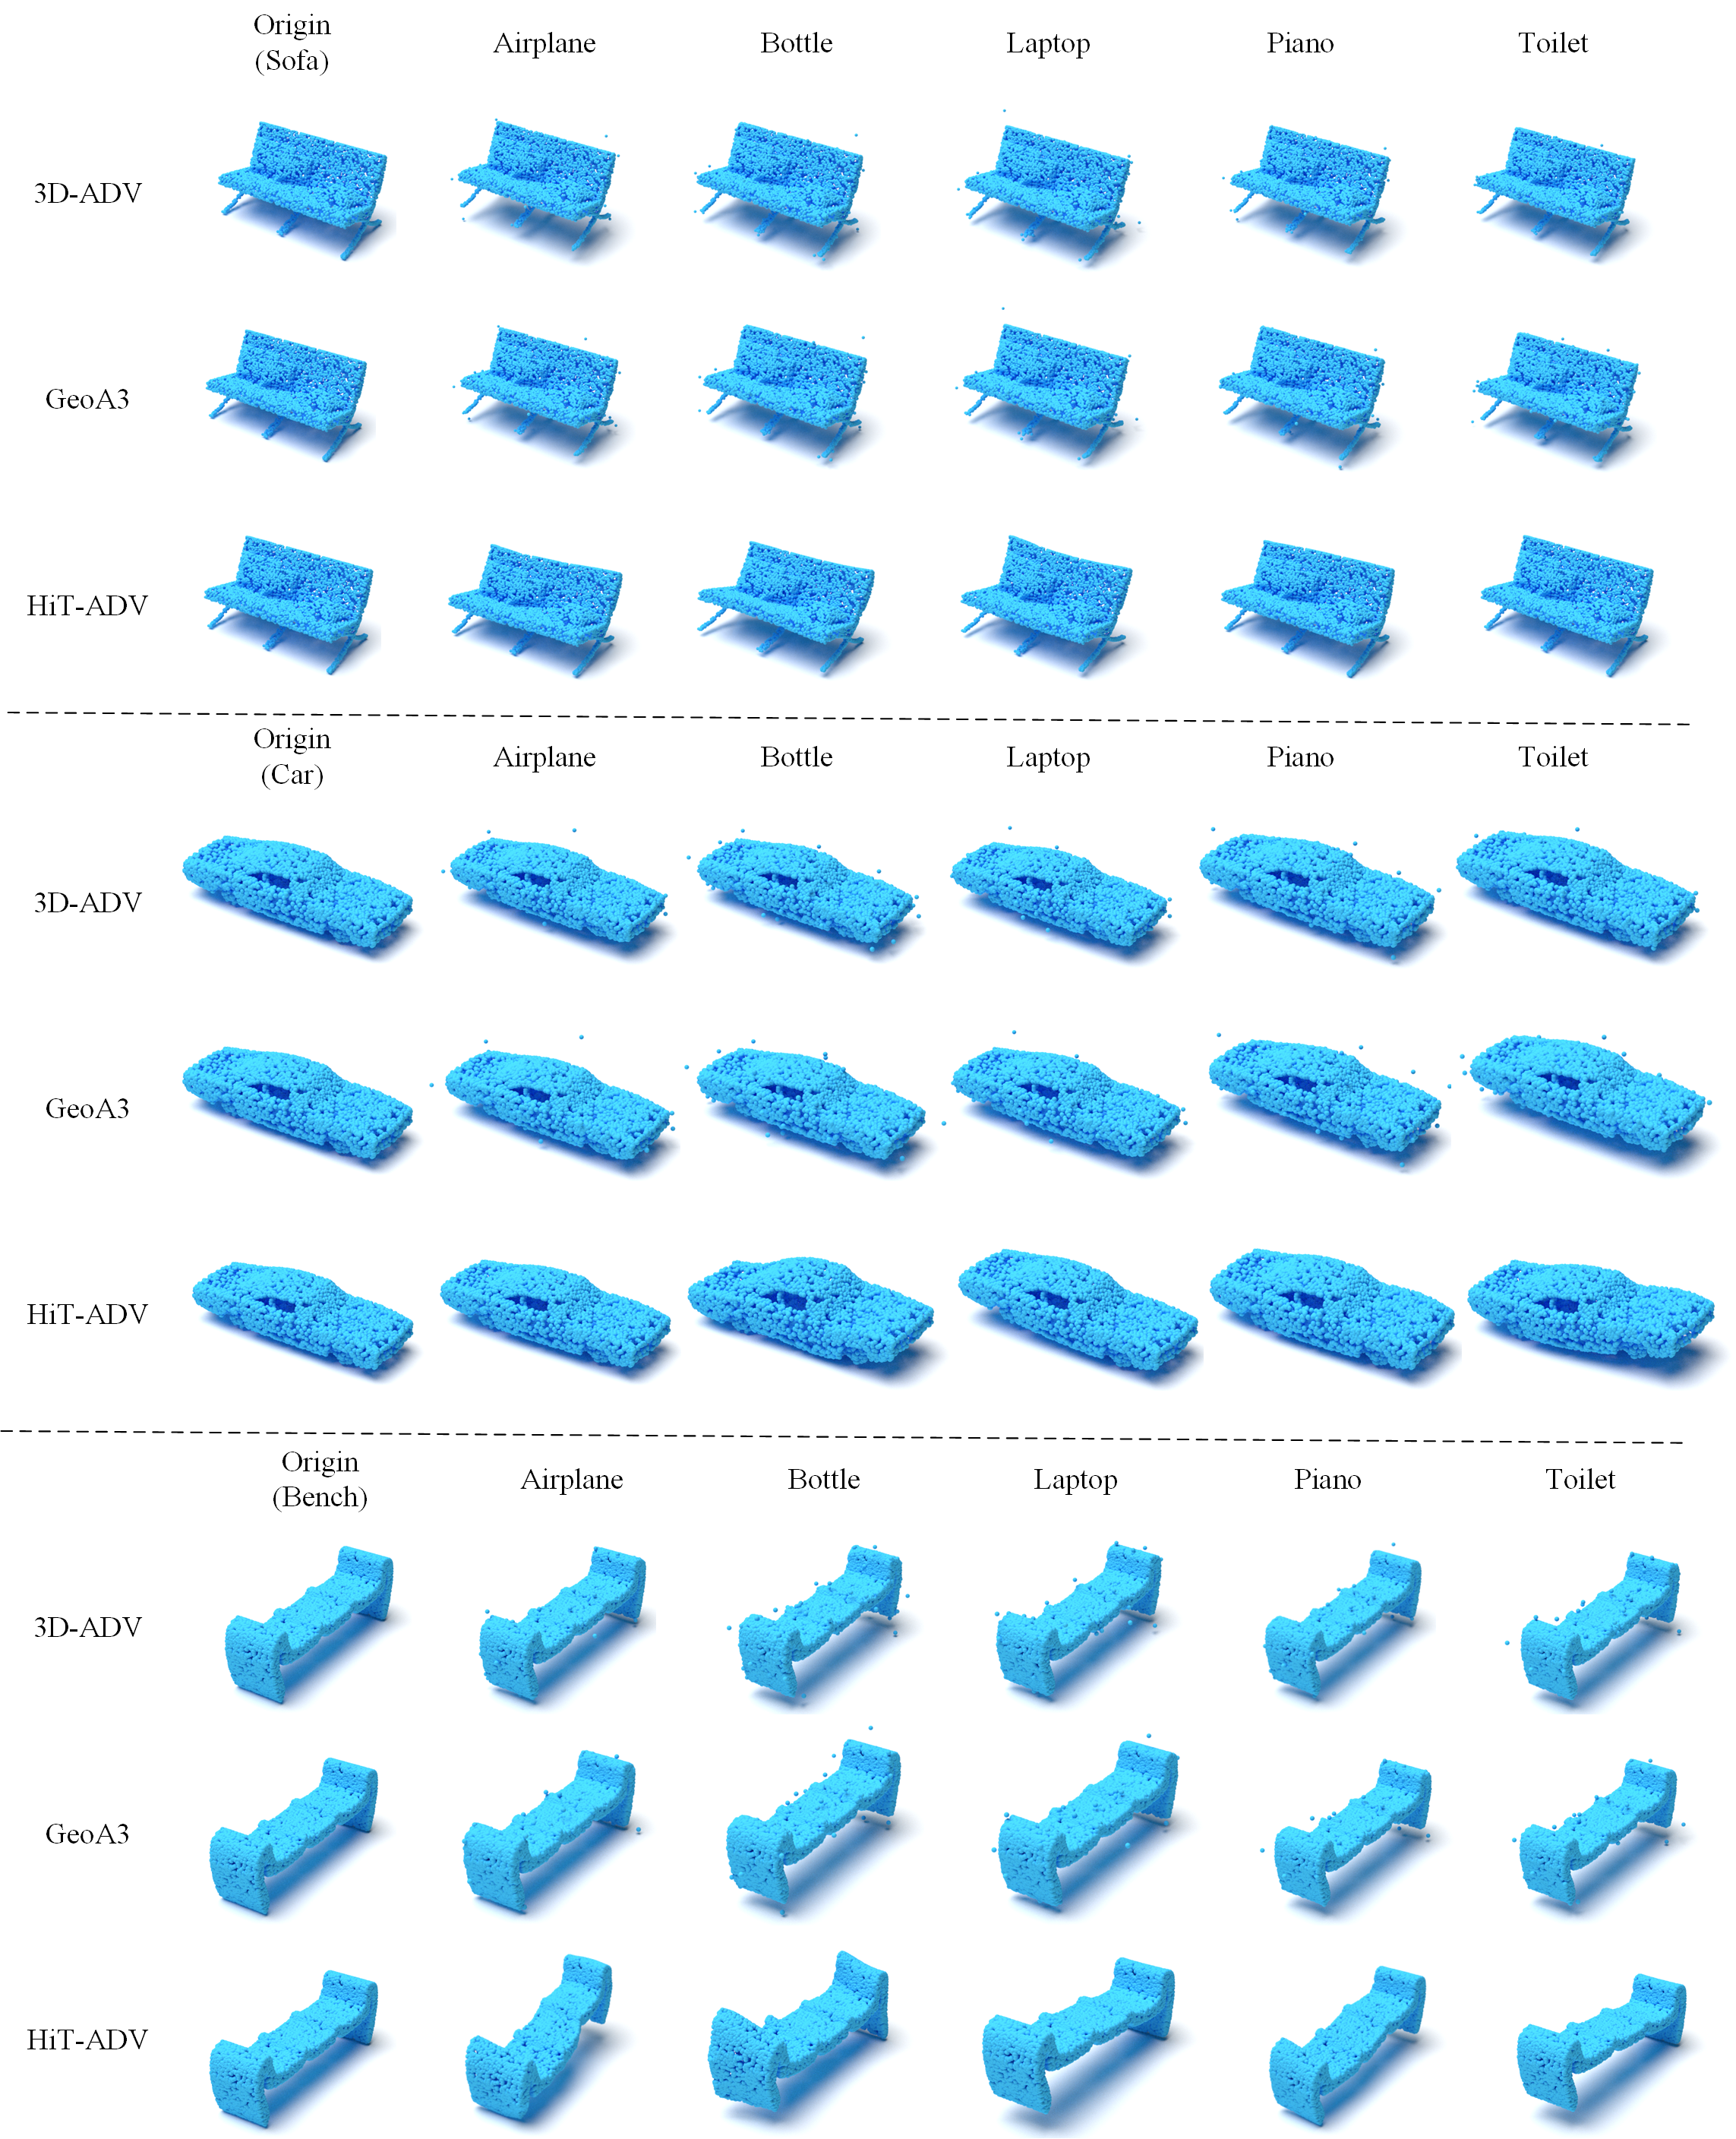}
   \caption{Visualization of original and adversarial point clouds generated by different targeted adversarial attack methods for attacking PointNet. We list the attack results of different target labels.}
   \label{fig:target}
   \vspace{-1mm}
\end{figure*}

\section{Supplement to Visualization Result}

To further demonstrate the effectiveness and superiority of HiT-ADV, we present more visualization comparisons of adversarial examples generated from ShapeNet Part dataset~\cite{chang2015shapenet} and different models~\cite{qi2017pointnet, wang2019dgcnn} in this section, as shown in Fig~\ref{fig:visual_appendix}.
It is obvious that HiT-ADV can achieve successful attacks while maintaining good imperceptibility across all these settings.

\begin{figure*}[t]
  \centering
  % \fbox{\rule{0pt}{2in} \rule{0.9\linewidth}{0pt}}
   \includegraphics[width=1\linewidth]{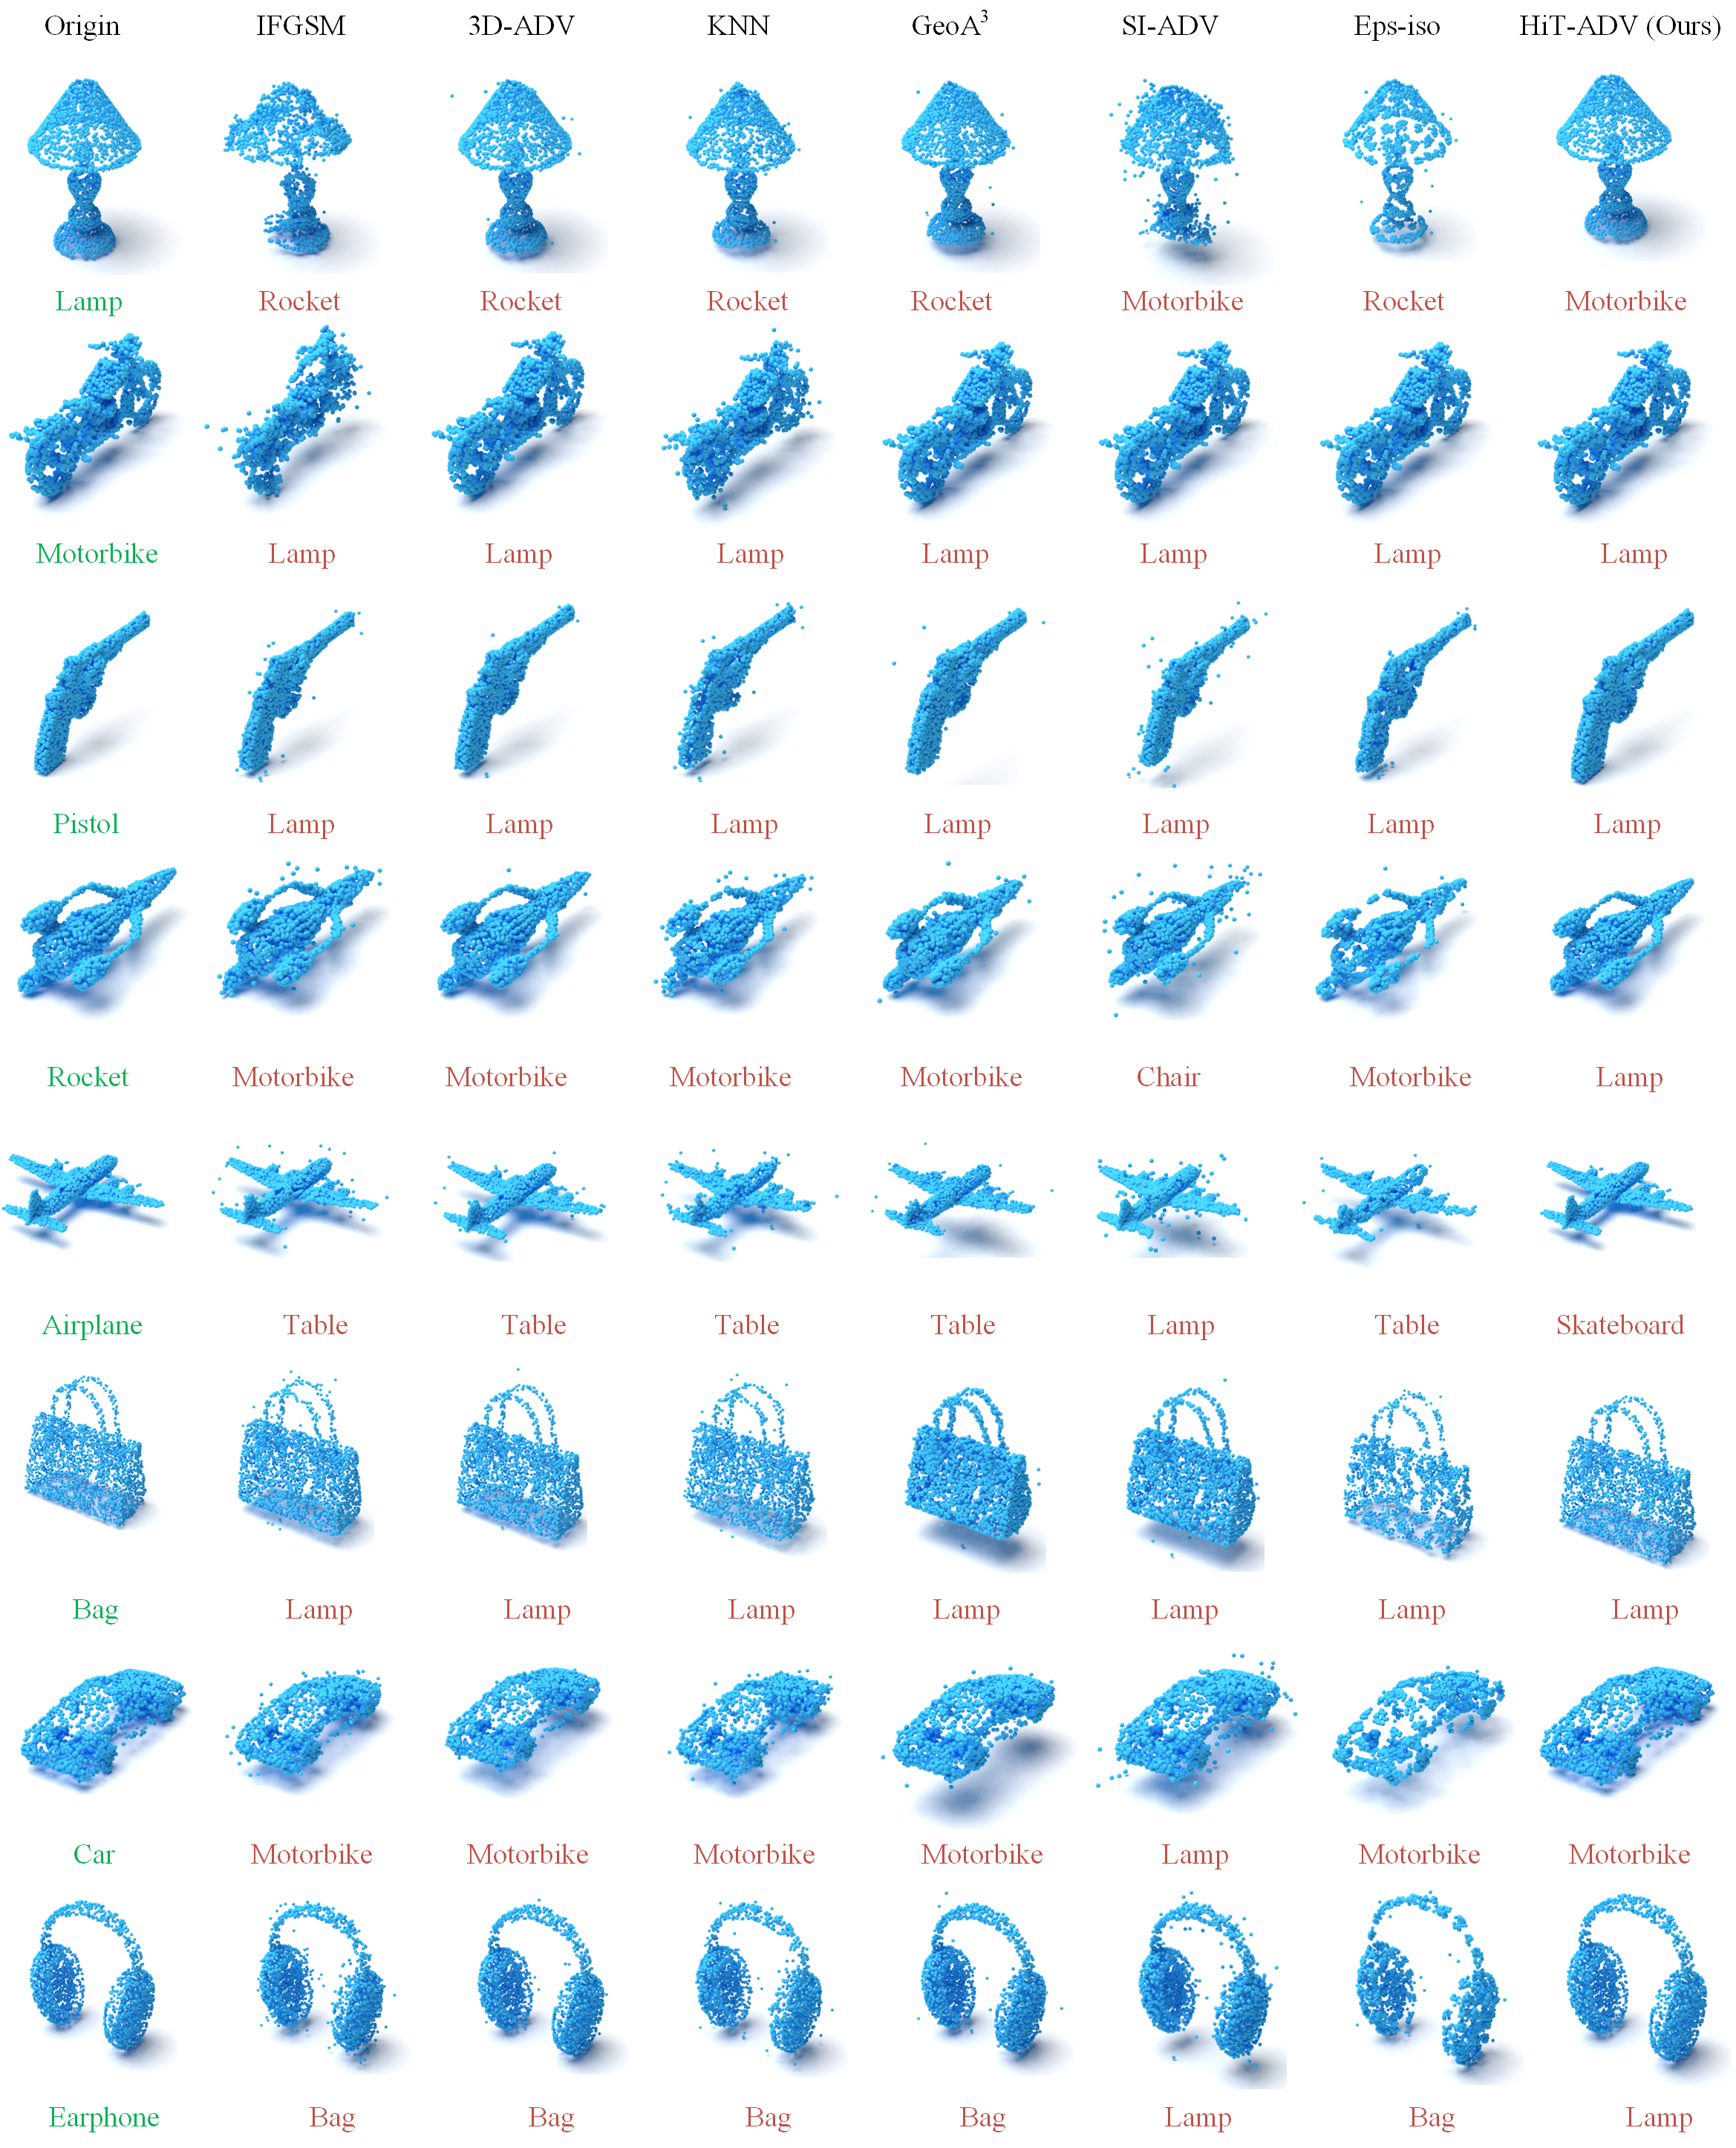}
   \caption{More visualization results of original and adversarial point clouds generated by different adversarial attack methods on the ShapeNet Part dataset. The first four rows show the results of attacking the DGCNN classification network, while the last four rows show the results of attacking the PointNet classification network.}
   \label{fig:visual_appendix}
   \vspace{-1mm}
\end{figure*}
